# Supplementary material for: HDMM: Optimizing error of high-dimensional statistical queries under differential privacy
Source: arXiv:2106.12118 source file (2021-06-23)
Supplement: Supplementary file 1 [file appendix_revised.tex]

\section{Appendix}

\subsection{Secondary Experiment: Utility} \label{sec:experiments_secondary}

\begin{table*}
\centering
\subcaptionbox{\label{tbl:marg-1d} 1D workloads}{
\resizebox{.48\textwidth}{!}{
\begin{tabular}{cc|SSSS|S}%{cc|ccccc|c}
\textbf{Workload}                        & \textbf{Domain} & \textbf{Identity} & \textbf{Wavelet} & \textbf{HB} & \textbf{GreedyH} & \textbf{\sys} \\\hline
\multirow{3}{1cm}{{All Range}}      & {128}    & 1.38         & 1.85             & 1.38        & \textbf{1.16}             & \textbf{\emph{1.00}}         \\
                                         & {1024}   & 2.36        & 1.83             & \textbf{1.16}        & 1.33             & \textbf{\emph{1.00}}         \\
                                         & {8192}   & 4.51    & 1.79             & \textbf{1.12}        & 1.67             & \textbf{\emph{1.00}}         \\\hline
\multirow{3}{1cm}{{Prefix}}         & {128}    & 1.80         & 1.78             & 1.80        & \textbf{1.20}             & \textbf{\emph{1.00}}         \\
                                         & {1024}   & 3.34        & 1.80             & \textbf{1.34}        & 1.49             & \textbf{\emph{1.00}}         \\
                                         & {8192}   & 6.40        & 1.70             & \textbf{1.20}        & 2.09             & \textbf{\emph{1.00}}         \\\hline
\multirow{3}{1cm}{{Permuted Range}} & {128}    & 1.38        & 4.67             & 1.38        & \textbf{1.35}             & \textbf{\emph{1.00}}         \\
                                         & {1024}   & 2.36       & 10.57            & 3.35        & \textbf{2.16}             & \textbf{\emph{1.00}}         \\
                                         & {8192}   & 4.52       & 25.85            & 9.34        & \textbf{3.82}             & \textbf{\emph{1.00}}
\end{tabular}
}
}%
\hfill
\subcaptionbox{\label{table:2drange} 2D workloads}{
\resizebox{.48\textwidth}{!}{
\begin{tabular}{cc|SSSS|S}
\textbf{Workload}                   & \textbf{Domain}      & \textbf{Identity} & \textbf{Wavelet}    & \textbf{HB} & \textbf{QuadTree} & \textbf{\sys} \\
\multirow{3}{*}{$\P \otimes \P$}                                   & {64 x 64}     & 2.35              & 3.40  & \textbf{1.41}     & 1.72     & \textbf{\emph{1.00}} \\
                                    & {256 x 256}   & 4.75              & 3.14  & 2.03     & \textbf{1.95}     & \textbf{\emph{1.00}} \\
                                    & {1024 x 1024} & 11.17             & 3.25  & 2.96     & \textbf{2.49}     & \textbf{\emph{1.00}} \\\hline
\multirow{3}{*}{$ \R \otimes \R$}                                    & {64 x 64}     & 1.54              & 3.59  & \textbf{1.45}     & 1.72     & \textbf{\emph{1.00}}  \\
                                    & {256 x 256}   & 2.64              & 3.37  & 1.91     & \textbf{1.79}     &  \textbf{\emph{1.00}} \\
                                    & {1024 x 1024} & 5.57              & 3.34  & 2.54     & \textbf{2.09}     & \textbf{\emph{1.00}} \\\hline
\multirow{3}{*}{$ \begin{bmatrix} \R \otimes \T \\ \T \otimes \R \end{bmatrix} $}                                    & {64 x 64}     & 5.00              & 7.00  & \textbf{3.51}     & 4.13     & \textbf{\emph{1.00}} \\
                                    & {256 x 256}   & 13.68             & 8.52  & 7.88     & \textbf{6.69}     & \textbf{\emph{1.00}} \\
                                    & {1024 x 1024} & 38.84             & \textbf{10.31} & 13.91    & 10.49    &  \textbf{\emph{1.00}} \\\hline
\multirow{3}{*}{$\begin{bmatrix} \P \otimes \I \\ \I \otimes \P \end{bmatrix}$}
                                   & {64 x 64}     & \textbf{1.11}              & 5.26  & 2.08     & 3.32     & \textbf{\emph{1.00}} \\
                                    & {256 x 256}   & \textbf{1.44}              & 6.11  & 4.05     & 4.71     & \textbf{\emph{1.00}} \\
                                    & {1024 x 1024} & \textbf{1.99}              & 6.79  & 7.27     & 6.81     & \textbf{\emph{1.00}} \\
\end{tabular}
} } \vspace{-1ex}
\caption{\label{tab:lowd} Error, {\em relative to \sys}, of (a) four competing methods evaluated on three one-dimensional workloads for varying domain sizes, and (b) of four competing methods on a variety of two-dimensional workloads. (Best competitor in {\bf bold}.)}
\end{table*}

In this section we look deeper into the utility of HDMM on one and two dimensional range query workloads, comparing it against other data-independent algorithms that are specifically designed to offer high utility in this setting.  We also look into the quality of strategies found by HDMM for 8 dimensional marginals workload.  %Then we consider a data-dependent algorithm, DAWA \cite{li2014data}, and show that its performance can be improved by using \sys.

We remind the reader that the error of the algorithms in this section do not depend on the data -- only the domain, and thus the error ratios that we report hold for all data vectors with the given domain.  

\paragraph*{One- and two-dimensional workloads}

The accuracy of \sys on low dimensional workloads is important because our methods decompose the optimization of high-dimensional workloads into single-dimensional sub-problems.  In addition, \sys can be used as a replacement for existing methods in low dimensions.   In this section we first compare \sys with a variety of data-independent algorithms, all of which fall into the select-measure-reconstruct paradigm.  Thus, we are comparing the strategy identified by \sys to the strategies that were manually crafted by algorithm designers to perform well on certain workloads.
We first evaluate \sys on range query workloads, comparing against existing data-independent algorithms designed specifically for such workloads: these are
%H2~\cite{hay2010boosting} (in 1D only),
Wavelet~\cite{xiao2011differential},
HB~\cite{qardaji2013differentially},
QuadTree~\cite{cormode2012differentially} (2D only),
and the only truly workload-adaptive technique,
GreedyH~\cite{li2014data} (1D only).
\cref{tbl:marg-1d} shows the results for 1D workloads, for which \sys has the lowest expected answer in all cases.  The margins of improvement are sometimes modest, we believe because, for 1D workloads, competing approaches have found close-to-optimal solutions.  Importantly, \sys beats the only available workload-adaptive method, GreedyH, which solves for optimal weights applied to a hierarchical strategy. The central assumption made by these methods is that the workload queries tend to exhibit locality, in that nearby elements of the domain are typically queried for together.  No such assumption is made by \sys, and the third workload (Permuted Range) highlights this: \sys is the only method that offers acceptable utility.  Permuted Range is a workload consisting of all range queries right-multiplied by a random permutation matrix, which serves to shuffle the elements of the domain.

%\ry{should more be said here?}

%The strategy produced by our method for all range queries has interesting and understandable structure.  Figure~\ref{fig:range_strategy} representes the strategy produced by the optimization for the workload of all range queries on a domain of size 256.  Most of the cells in each query are zero, the non-zero cells are all contiguous, and the values of the non-zero cells increase towards the middle and decrease towards the endpoints of the contiguous region.  Upon reflection, this behavior is somewhat intuitive - each of the non-trivial query is used to answer many range queries, but it is most useful for answering range queries that are centered in the same region of the domain.  By understanding this structure for small domains, we could in principle approximately solve the optimization problem for larger domains where the optimization is intractable to do directly.

%\begin{figure}
%\includegraphics[width=\linewidth]{fig/viz256.pdf}
%\caption{ \label{fig:range_strategy} A visual depiction of the optimized strategy for a workload of all range queries on a domain of size 256 (using Problem 2).  Each row of the graph represents one of the $p=13$ non-Identity queries.  The $x$-axis represents the cells in the data vector and the $y$-axis represents the weight on that cell in the query.  The identity queries are not plotted, since weights on those queries can be derived from the non-Identity weights.}
%\end{figure}
For 2D workloads, \cref{table:2drange} shows that \sys outperforms all data-independent competitors on various workloads composed from Range, Prefix and unions thereof. In addition, the error improvements offered by \sys are more substantial (as much as 10$\times$), suggesting that they grow as the number of dimensions increases.

    Importantly, without \sys, to achieve the best error rates for these 1D and 2D tasks, one has to choose between many algorithms (Wavelet, HB, GreedyH, Quadtree) each of which is best for some workload; \sys can replace them all  and improves error uniformly.

%Now we analyze the effectiveness of our methods on three 2D range query workloads, and again show that our method outperforms all competitors.  There are two sources of improvement from using our method.  First is the realization that the strategy should be expressible as a Kronecker product.  Existing approaches such as HB produce strategies that are not Kronecker products in general (except in the degenerate case when HB = Identity), meaning we would be better off taking the Kronecker product of two 1D HB strategies than using the 2D HB strategy.  The second source of improvement comes from the fact that our methods are the best on the 1D sub-problems, and this improvement in 1D is magnified in higher dimensions as the error ratio grows geometrically.

%We also use the 2D Random Range query workload to test the projection heuristic described in section~\ref{sec:projection}, as this workload cannot in general be represented as a Kronecker product, and the workload is too big to optimize directly when the size of each dimension exceeds 64.

%All of the 1D strategies in table~\ref{table:range} can be lifted into a 2D strategy by taking the Kronecker product, and we can easily reason about the RMSE analytically by referring to proposition~\ref{prop:decomposition}.  For example, the workload of all 2D range queries on a $128 \times 128$ domain, OptAllRange will still have the best RMSE, and GreedyH, which is the best competing alternative, will have a relative RMSE of $ 1.16^2 \approx 1.35 $, and the improvements continue to grow with the dimensionality.

\paragraph*{Marginals Workloads}

We now evaluate \sys on $8$-dimen\-sional data where each attribute domain has size 10, so that $N=10^8$.  Workloads are defined by $K$ where for a given $K$, the workload includes all $i$-way marginals where $i \leq K$. We compare \sys with three techniques: \Identity, \LMW and DataCube~\cite{ding2011differentially}.
\begin{table}[h!]
\centering
\resizebox{.4\textwidth}{!}{
\begin{tabular}{r|SSS|c}
\textbf{Workload} & \multicolumn{1}{c}{\textbf{\Identity}} & \multicolumn{1}{c}{\textbf{\LMW}} & \multicolumn{1}{c}{DataCube} & \sys \\\hline
%$K=0$ & \textbf{\emph{1.00}}0.00          & \textbf{\emph{1.00}}            & \textbf{\emph{1.00}} & \textbf{\emph{1.00}}         \\
$K=1$ & 435.19            & 1.18              & \textbf{1.12} & \textbf{\emph{1.00}}         \\
{2} & 43.89             & 1.43              & \textbf{1.03} & \textbf{\emph{1.00}}         \\
{3} & 8.37              & 1.96              & \textbf{1.15} & \textbf{\emph{1.00}}         \\
{4} & 2.73              & 3.03              & \textbf{1.21} & \textbf{\emph{1.00}}         \\
{5} & \textbf{1.33}              & 4.95              & 1.36 & \textbf{\emph{1.00}}         \\
{6} & \textbf{\emph{1.00}}              & 9.21              & 1.67 & \textbf{\emph{1.00}}         \\
{7} & \textbf{1.07}              & 18.21             & 2.99 & \textbf{\emph{1.00}}         \\
{8} & \textbf{1.06}              & 24.94             & 5.76 & \textbf{\emph{1.00}}
\end{tabular}
} \vspace{-1ex}
\caption{\label{tab:highd_marginals} Error, measured as \errRatio, on workloads of all up-to-$K$-way marginals on domain size of $10^8$.
}
\end{table}

As shown in \cref{tab:highd_marginals}, \sys outperforms the baselines in all target settings; the magnitude of the improvement depends on $K$.  \LMW is nearly optimal for small $K$, whereas \Identity is nearly optimal for large $K$, but \sys improves on both substantially for $K=3,4,5$.  For each experimental setting, one or the other baseline provides low error. But we emphasize the value of fully automated optimization: the algorithm designer is not forced to select the appropriate baseline, which will vary with domain size and workload.  %The poor performance of DataCube for large $K$ is likely due to the fact that it optimizes for a different error metric (maximum rather than average error).

\subsection{Improving the DAWA Algorithm}

\begin{table}[h]
\centering
\resizebox{0.8\columnwidth}{!}{
\begin{tabular}{c|ccc|ccc|}
\multirow{2}{1.2cm}{{\bf domain \\ size}}&   \multicolumn{3}{c|}{{\bf data size} = 1000} & \multicolumn{3}{c|}{{\bf data size} = 10000000} \\
 & \textbf{min} & \textbf{median} & \textbf{max} & \textbf{min} & \textbf{median} & \textbf{max}\\\hline
 256             & 1.04         & 1.12            & 1.7          & 1.18         & 1.25            & 1.44         \\
 1024            & 1.04         & 1.15            & 1.91         & 1.15         & 1.37            & 1.92         \\
 4096            & 1.08         & 1.20             & 1.84         & 1.45         & 1.80             & 2.28 \\ \hline
\end{tabular} }
\caption{\label{table:dawa} Error ratio between modified DAWA and original DAWA. Min/median/max error across 5 datasets (Hepth, Medcost, Nettrace, Patent, Searchlogs~\cite{hay2016principled}) conforming to three domain sizes and two data sizes ($\epsilon=\sqrt{2}$).}
\end{table}
In the empirical study performed by Hay et al. \cite{hay2016principled}, the DAWA algorithm~\cite{li2014data} was one of the best performing algorithms for 1D and 2D linear query workloads.  The algorithm is data-dependent, using part of the privacy budget in a first stage that finds a partition of the data into uniform contiguous regions that are well-approximated by uniformity. The second stage of the algorithm, is an instance of the select-measure-reconstruct pattern which uses GreedyH (described above).  To show the value of \sys in improving the state-of-the-art, we modify DAWA by replacing GreedyH with \sys and measured the impact.  Since DAWA is data-independent, we use a range of datasets and dataset sizes taken from \cite{hay2016principled} for the evaluation.  The workload is Prefix, which is a workload that GreedyH was designed to support.

To evaluate the impact, we measure the ratio of error between the modified algorithm and the original DAWA.  \cref{table:dawa} reports the min, median, and max improvement to GreedyH across the 5 datasets.  Maximum error improvements approach a factor of 2 in many cases; an impressive result considering that DAWA has been carefully tuned and outperforms most other algorithms in the literature.
