# Supplementary material for: HDMM: Optimizing error of high-dimensional statistical queries under differential privacy
Source: arXiv:2106.12118 source file (2021-06-23)
Supplement: Supplementary file 2 [file appendix_old.tex]

\section{Section 5 proofs}
\subsection{Proof of Formula~\ref{eq:grad}}

In section~\ref{sec:optimization}, we made the following claim:

\begin{equation}
\begin{aligned}
\frac{\partial C}{\partial \A} &= -2 \A (\A^T \A)^+ (\W^T \W) (\A^T \A)^+
\end{aligned} \tag{\ref{eq:grad}}
\end{equation}

First note that $C(\A)$ can be expressed as $tr[\X^+ \Y]$ where $\X = \A^T \A$ and $\Y = \W^T \W$  From matrix calculus~\cite{peterson2008matrix}, we know that $ \frac{\partial C}{\partial \X} = -\X^{-1} \Y \X^{-1} $ if $ \X $ is invertible, and more generally
$$ \frac{\partial C}{\partial \X} = -\X^+ \Y \X^+ + (\X^+ \X^{+T}) \Y (\I - \X \X^+) + (\I - \X^+ \X) \Y (\X^{+T} \X^+) $$
which simplifies to $ \frac{\partial C}{\partial \X} = -\X^+ \Y \X^+ = -(\A^T \A)^+ (\W^T \W) (\A^T \A)^+ $ when $\A$ supports $\W$.

%If $A$ supports $W$, then $ W = W A^+ A $ by definition, and it follows immediately that $ W^T W = W^ (W A^+ A) $.  Furthermore, $ A^+ = (A^T A)^+ A^T $, so $ A^+ A = X^+ X = X X^+ $ since $X$ and $X^+$ are symmetric.  It follows that $ Y = Y X X^+ $ and $ Y = X^+ X Y $.  Plugging this result into the original equation shows the first desired result holds in general (as long as $A$ supports $W$).

%\begin{align*}
%\frac{\partial tr[X^+ Y]}{\partial X} &= -X^+ Y X^+ + (X^+ X^{+T}) (Y - Y X X^+) + (Y - X^+ X Y) (X^{+T} X^+)\\
%&= -X^+ Y X^+ + (X^+ X^{+T}) 0 + 0 (X^{+T} X^+)\\
%&= -X^+ Y X^+
%\end{align*}

The gradient of $C$ with respect to $\A$ can be written in terms of the gradient of $C'$ with respect to $\X$ using the chain rule:

\begin{align*}
\frac{\partial C}{\partial \A} &= 2 \A \frac{\partial C'}{\partial \X} \\
&= -2 \A (\A^T \A)^+ (\W^T \W) (\A^T \A)^+
\end{align*}

Thus, the claim holds (as long as $\A$ supports $\W$).  

Note that in order to apply gradient based optimization with respect to a parameterized strategy $\A(\vect{\theta})$, it is necessary to apply the chain rule again:
$$ \frac{\partial C}{\partial \theta_k} = \sum_{i,j} \frac{\partial C}{\partial A_{ij}} \frac{\partial A_{ij}}{\partial \theta_k} $$
depending on the parameterization, this may or may not be expressible compactly in terms of matrix operations.  

\subsection{Analysis of $\optgp$}

Below is the proof of \cref{thm:optgp} showing the complexity of the objective and its gradient for $\optgp$.

\thmoptgp

\begin{proof}
Assume $\W^T \W$ has been precomputed
%\gm{do we need to say something about this upfront?}
and now express $ \A^T \A $ in terms of $\matr{\Theta}$ and $\D$:
$$ \A^T \A = \D^T \D + \D^T \matr{\Theta}^T \matr{\Theta} \D = \D[\I_n + \matr{\Theta}^T \matr{\Theta}] \D $$
Applying the identity $ (\X \matr{Y})^{-1} = \matr{Y}^{-1} \X^{-1} $ together with the Woodbury identity~\cite{hager1989updating} yields an expression for the inverse:
%
\begin{align*}
(\A^T \A)^{-1} &= \D^{-1} [\I_n + \matr{\Theta}^T \matr{\Theta}]^{-1} \D^{-1} \\
&= \D^{-1} [\I_n - \matr{\Theta}^T (\I_p + \matr{\Theta} \matr{\Theta}^T)^{-1} \matr{\Theta}] \D^{-1}
\end{align*}

We can compute $ (\A^T \A)^{-1} (\W^T \W) $ in $O(n^2 p)$ time by evaluating the following expression from right to left:
$$ (\A^T \A)^{-1} (\W^T \W) = \D^{-2} (\W^T \W) - \D^{-1} \matr{\Theta}^T (\I_p + \matr{\Theta} \matr{\Theta}^T)^{-1} \matr{\Theta} \D^{-1} (\W^T \W)  $$

By carefully looking at the dimensionality of the intermediate matrices that arise from carrying out the matrix multiplications from right-to-left, we see that the most expensive operation is the matrix-matrix product between an $ n \times p$ matrix and a $p \times n$ matrix, which takes $O(n^2 p)$ time.  The inverse $ (\I_p + \matr{\Theta} \matr{\Theta}^T)^{-1} $ takes $O(p^3)$ time and the operations involving $D$ take $O(n^2)$ time since it is a diagonal matrix.

The result still holds even if $\W^T \W$ is replaced with an arbitrary $n \times n$ matrix, so $ \X = (\A^T \A)^{-1} (\W^T \W) (\A^T \A)^{-1} $ can be computed in $O(n^2 p)$ time as well.  The gradient is $ -2 \A \X $ whose components can be calculated separately as $ -2 \D \X $ and $ -2 \Theta \X $.  $ -2 \D \X $ takes $O(n^2)$ time and $ \matr{\Theta} \X$  takes $O(n^2 p)$ time, so the overall cost of computing the gradient is $O(n^2 p)$.
\end{proof}

\subsubsection*{Fast Measure and Reconstruct with $p$-Identity strategies}

Because $\optgp$ is only really tractable for domains where $n \leq 8192$, we can run the mechanism directly in $O(n^3)$ time simply by using dense linear algebra.  However, we can improve that to $O(n p)$ by exploiting structure of the strategy and using the same techniques proposed in the proof of theorem~\ref{thm:optgp}.

\begin{algorithm}
\caption{Implicit Pseudo Inverse} \label{alg:pinv}
{\small
\begin{algorithmic}[1]
\Procedure{Pinv}{$\Theta$}
\State $p,n = $ \Call{shape}{$\Theta$}
\State $D^{-1} = $ \Call{diag}{\Call{ones}{$1$,$p$} $\Theta$}
\State $D = $ \Call{inv}{$D^{-1}$}
\State $M = $ \Call{inv}{$I_p + \Theta \Theta^T$}
\Procedure{Dot}{$y$} \Comment $A^+ y = (A^T A)^{-1} A^T y$
\State $ y = \begin{bmatrix} y^{(1)} \\ y^{(2)} \end{bmatrix} $
\State $ u = D (y^{(1)} + \Theta^T y^{(2)})$ \Comment $ A^T y $
\State \Return $ D^{-1} D^{-1} u - D^{-1} \Theta^T (M (\Theta D^{-1} u)) $  \Comment $ (A^T A)^{-1} a $
\EndProcedure

\State \Return \Call{ImplicitMatrix}{Dot}
\EndProcedure
\end{algorithmic}}
\end{algorithm}

\noindent \textbf{Measure}

Since $\A$ has at most $n (p+1)$ non-zero entries, the matrix-vector product $\A \x$ can be efficiently computed in $O(n p)$ time using sparse matrices.

\noindent \textbf{Reconstruct}

Solving the least squares problem requires computing $ \A^+ \vect{y} $ where $\vect{y}$ is the vector of private strategy query answers.  Since $\A$ has full column rank, $\A^+ = (\A^T \A)^{-1} \A^T$.  Using the sames ideas from the proof of theorem~\ref{thm:optgp}, we can compute $\A^+ \vect{y}$ in $O(n p)$ time by expressing the matrix-vector product in terms of $\matr{\Theta}$ and $\D$ and evaluating the resulting expression from right-to-left.  An implementation of this procedure is shown in algorithm~\ref{alg:pinv}.

\section{Section 6 proofs and extra material}

\thmerrdecomp

\begin{proof}[(Sketch)]
Recall from \cref{def:error} that the error of any workload under a strategy is:
	$$\text{Error}(\W, \A) =  || \A ||_1^2 || \W \A^+ ||_F^2$$
The theorem follows from the fact that the sensitivity of a Kronecker product is the product of the sensitivities of its sub-matrices (as shown in \cref{thm:kron-sens}) and the fact that:
$$ || (\W_1 \otimes \dots \otimes \W_d)(\A_1 \otimes \dots \otimes \A_d)^+  ||_F = \prod_{i=1}^d || \W_i\A_i^+  ||_F $$
\end{proof}


\subsection{sum-of-krons 2} \label{sec:sub:sumkrons2}
\gm{moved from parameterizations section}
Here we describe an approach to approximate the strategy that we want in these cases where parameterization~\ref{sec:sub:unionkron} isn't designed (e.g., not much overlap between between the queries in the subworkloads).  Consider workloads of the form shown in equation~\ref{eq:wsum}.  Now let $ A^{(j)} = A^{(j)}_1 \otimes \dots \otimes A^{(j)}_d $ denote the strategy optimized for $W^{(j)} = w_j (W_1^{(j)} \otimes \dots \otimes W_d^{(j)})$.  We then use the strategy defined below:

$$ A = \begin{bmatrix} a_1 (A^{(1)}_1 \otimes \dots \otimes A^{(1)}_d) \\ \vdots \\ a_k (A^{(k)}_1 \otimes \dots \otimes A^{(k)}_d) \end{bmatrix} $$

where $ \sum_{j=1}^k a_j = 1 $ and we can think of $a_j$ as the fraction of the privacy budget that we allocate to measuring the queries in $A^{(j)}$.  We already know how to find $ A^{(j)}$ using the techniques described in section~\ref{sec:sub:single-kron} and ~\ref{sec:sub:unionkron}, but we still need a method to find $a_j$.

First note that the error on the workload is equal to:

$$ || W A^+ ||_F^2 = \sum_{j=1}^k || W^{(j)} A^+ ||_F $$

but since $ A $ is a sum of kronecker products, $A^+$ doesn't decompose, and since the domain size is assumed to be large, it is infeasible to calculate computationally as well.  An upper bound on the error is given by
\begin{align*}
|| W A^+ ||_F^2 &\leq \sum_{j=1}^k || W^{(j)} (a_j A^{(j)})^+ ||_F^2 \\
&= \sum_{j=1}^k \frac{1}{a_j^2} || W^{(j)} A^{+(j)} ||_F^2
\end{align*}
and this upper bound is tight as long as there is not too much overlap between $ W^{(j)}$ and $ W^{(j')}$ for $j \neq j'$.  If there is a lot of overlap between $W^{(j)}$ and $W^{(j')}$ then they should be merged together into a single group and optimized together.  This upper bound is computationally tractable to compute, since $ || W^{(j)} A^{+(j)} ||_F^2 $ decomposes into a product of $d$ terms.

The resulting optimization problem is to find the $a_j$ that minimizes the upper bound on error.  As it happens, this problem has a closed form solution.  Note that $ || W^{(j)} A^{+(j)} ||_F^2 $ is just a constant that we have access to (as it was returned by the optimization that produced $A^{(j)})$, let's call it $C_j$.  Then the optimization problem that needs to be solved is

\begin{equation*}
\begin{aligned}
& \underset{\vec{a} \in \mathbb{R}^k_+}{\text{minimize}}
& & \sum_{j=1}^k \frac{C_j}{a_j^2} \\
& \text{subject to} & & \sum_{j=1}^k a_j = 1
\end{aligned}
\end{equation*}

The solution to this problem is

$$ a_j \propto (2 C_j)^{1/3} $$

For the slightly different workload,

$$ W = \begin{bmatrix} R \otimes I \\ I \otimes R \end{bmatrix} $$, we expect the original parameterization to perform reasonably well, but this one to perform poorly.  This is because there is much more overlap between the two query sets.  If we use the method proposed in this section, the resuling strategy would contain many duplicate copies of identity queries, which we know is suboptimal (that's not a problem in the first workload, since the weight on the identity queries would be near-zero).


\subsection{Marginals parameterization}

It is useful to formally define a correspondence between the integers $ [2^d] = \set{0, \dots, 2^d-1} $ and the query matrices for each marginal.  We therefore define $ \M : [2^d] \rightarrow \mathbb{R}^{n \times n} $ as follows:
%
$$ \M(a) = \bigotimes_{i=1}^d [\matr{1} (a_i = 0) + \I (a_i = 1)] $$
%
where $(a_i = 0)$ and $(a_i = 1)$ are indicator functions on the $i^{th}$ bit of the binary representation of $a$ and $\matr{1} = \T^T \T$ is the $n_i \times n_i$ matrix of ones.

We also define $\mathcal{M} : \mathbb{R}^{2^d} \rightarrow \mathbb{R}^{n \times n}$ as follows:
%
$$ \matr{\mathcal{M}}(v) = \sum_{a \in [2^d]} v_a M(a) $$
%
and note that $\W^T \W = \matr{\mathcal{M}}(w^2)$ and $ \A^T \A = \matr{\mathcal{M}}(\theta^2)$ for a marginals strategy and workload. 
%Since the sensitivity of a strategy is $ \sum \theta_i $ assuming $\theta_i \geq 0$, the optimization problem can be formulated as:

\begin{example}
For a 3 dimensional domain the query matrix for a 2 way marginal can be expressed as $ \matr{Q} = \I \otimes \T \otimes \I $, and $\matr{Q}^T \matr{Q} = \I \otimes \matr{1} \otimes \I = \M(101_2) = \M(5) $.
\end{example}

Proposition~\ref{prop:marginals} shows that matrices $\M(a)$ and $\M(b)$ interact nicely under matrix multiplication.

\begin{proposition} \label{prop:marginals}
For any $a, b \in [2^d] $, $$\M(a) \M(b) = C(a | b) \M(a \& b)$$ where $ a | b $ denotes ``bitwise or'', $ a \& b $ denotes ``bitwise and'', and $C(k) = \prod_{i=1}^d n_i (k_i = 0)$.
\end{proposition}

\begin{proof}
First observe how the matrices $\I$ and $\matr{1}$ interact under matrix multiplication:
\begin{align*}
\I \I = \I && \I \matr{1} = \matr{1} && \matr{1} \I = \matr{1} && \matr{1} \matr{1} = n_i \matr{1} \\
\end{align*}
Now consider the product $\M(a) \M(b)$ which is simplified using Kronecker product identities, logical rules, and bitwise manipulation.
\begin{align*}
&= \bigotimes_{i=1}^d [\matr{1} (a_i = 0) + \I (a_i = 1)] [\matr{1} (b_i = 0) + \I (b_i = 1)]  \\
&= \bigotimes_{i=1}^d n_i (a_i = 0 \text{ and } b_i = 0) [\matr{1} (a_i = 0 \text{ or } b_i = 0) + \I (a_i = 1 \text{ and } b_i = 1)] \\
&= \bigotimes_{i=1}^d n_i ( (a | b)_i = 0) [\matr{1} ( (a \& b)_i = 0) + \I ( (a \& b)_i = 1)] \\
&= C(a|b) \M(a \& b)
\end{align*}
\end{proof}

From proposition~\ref{prop:marginals}, it follows that $ \set{c \matr{\mathcal{M}}(v) \mid c \in \mathbb{R}, v \in \mathbb{R}^{2^d}}$ is closed under matrix multiplication.  In fact, the relationship is linear: for fixed $u$, the product $ \matr{\mathcal{M}}(u) \matr{\mathcal{M}}(v) $ is linear in $v$.

\begin{proposition} \label{prop:marginals2}
For any $u, v \in \mathbb{R}^{2^d}$, $\matr{\mathcal{M}}(u) \matr{\mathcal{M}}(v) = \matr{\mathcal{M}}(\X(u) v)$ where $\X(u)$ is a triangular matrix (a linear map) that depends on $u$.
\end{proposition}

\begin{proof}
Let $u, v \in \mathbb{R}^{2^d}$ and consider the following product:
\begin{align*}
\matr{\mathcal{M}}(u) \matr{\mathcal{M}}(v) &= \Big( \sum_a u_a \M(a) \Big) \Big( \sum_b v_b \M(b) \Big) \\
&= \sum_{a,b} u_a v_b \M(a) \M(b) \\
&= \sum_{a,b} u_a v_b C(a | b) \M(a \& b) \\
\end{align*}
Observe that $ \matr{\mathcal{M}}(u) \matr{\mathcal{M}}(v) = \matr{\mathcal{M}}(w) $ where
$$ w_k = \sum_{a \& b = k} u_a v_b C(a | b) $$
The relationship between $w$ and $v$ is clearly linear, and by carefully inspecting the exression one can see that $ w = \X(u) v $ where $ \X(u)[k,b] = \sum_{a : a \& b = k} u_a C(a | b) $.  $\X(u)$ is an upper triangular matrix because $k = a\&b$ and $ a \& b \leq b$ for all $a$.
\end{proof}

We can use proposition~\ref{prop:marginals2} to efficiently multiply two matrices of this form in the compact representation, and we can also apply it to find the inverse or a generalized inverse of a matrix of this form.  In particular, if $v$ is a solution to the linear system $\X(u) v = z$ where $\matr{\mathcal{M}}(z) = \I $ then $ \matr{\mathcal{M}}(u)^{-1} = \matr{\mathcal{M}}(v) $.  A similar linear system can be solved to find a generalized inverse or the pseudo inverse if $ \matr{\mathcal{M}}(u) $ is not invertible.

This gives us all the machinery we need to efficiently compute the objective function using the trace formulation, since $ \matr{\mathcal{M}}(v) = \matr{\mathcal{M}}(w^2) \matr{\mathcal{M}}(\theta^2)^+ $, and $tr[\matr{\mathcal{M}}(v)] = n \sum v_a $

%%%%%%%%%%%%%%%%%%%%%%%%%%%%%%%%%%%%%%%%%%%%%%%%%%%%%%%%
\section{Other stuff}
\subsection{Matrix-Vector Products}

The algorithm described in section ~\ref{sec:running} for computing $ \AA \x $ without materializing $\AA$ is shown formally in algorithm~\ref{alg:ikron}.

\begin{algorithm}
\caption{Implicit Kronecker Products} \label{alg:ikron}
{\small
\begin{algorithmic}[1]
\Procedure{Kron}{$A$, $B$}
\State $ m_1, n_1 = $ \Call{shape}{$A$}
\State $ m_2, n_2 = $ \Call{shape}{$B$}
\Procedure{Dot}{$x$}
\State $ X = $ \Call{mat}{$x$, $n_1 \times n_2$}
\State \Return \Call{vec}{$A X B^T$}
\EndProcedure
\State \Return \Call{ImplicitMatrix}{Dot}
\EndProcedure
\item[]
\Procedure{Krons}{$A_1, \dots, A_d$}
\State \Return \Call{fold}{Kron, [$A_1, \dots, A_d$]}
\EndProcedure
\item[]
%\Procedure{Pinv Krons}{$\Theta_1, \dots, \Theta_d$}
%\State \Return \Call{Krons}{\Call{Pinv}{$\Theta_1$}, $\dots$, \Call{Pinv}{$\Theta_d$}}
%\EndProcedure
\end{algorithmic}}
\end{algorithm}

Algorithm~\ref{alg:ikron} is fast theoretically and simple conceptually, but slow in practice.  Algorithm~\ref{alg:fastikron} shows a carefully vectorized implementation that is much faster in practice.

\begin{algorithm}
\caption{Implicit Kronecker Products} \label{alg:fastikron}
{\small
\begin{algorithmic}[1]
\Procedure{Krons}{$A_1, \dots, A_d$}
\State $N = \prod_{i=1}^d$ \Call{cols}{$A_i$}
\State $m_i, n_i = $ \Call{shape}{$A_i$}
\Procedure{Dot}{$x$}
\State $Y_d = x$
\State $N_d = N$
\For{$i = d, \dots, 1$}
\State $Z_i = $ \Call{transpose}{\Call{reshape}{$Y_i$, $N_i/n_i$, $n_i$}}
\State $Y_{i-1} = A_i Z_i$
\State $N_{i-1} = N_i * m_i / n_i$
\EndFor
\State \Return \Call{vec}{$Y_0$}
\EndProcedure
\State \Return \Call{ImplicitMatrix}{Dot}
\EndProcedure
\end{algorithmic}}
\end{algorithm}

%\subsection{Auxilary Information} \gm{I moved this out of body of the paper because I'm not sure we need it.}

%In this section we introduce a simple technique to handle the strategy optimization problem in the prescence of background information.  This can be noisy background information, such as noisy linear query answers obtained previously, or non-noisy information such as known totals and structural zeros.  To do that, we modify the objective function to account for the background information.

%Assume we have noisy answers to a set of linear queries $B$, a workload $W$, and we want to find a strategy $A$ for $W$ that accounts for the fixed measured information we obtained from $B$.  Assuming the rows of $A$ and $B$ are scaled so that the noisy answers have variance $1$, the expected workload query answers after applying least-squares is
%$$ || W \begin{bmatrix} A \\ B \end{bmatrix}^+ ||_F^2 = tr[(A^T A + B^T B)^+ (W^T W)] $$
%By optimizing with respect to this objective function, as opposed to $ || W A^+ ||_F^2 $, we can find higher quality strategies that use the auxilery information correctly.  The validity of this formula relies on the assumption that the queries in $A$ and $B$ are answered with the same noise variance.

%Encoding non-noisy background information is straightforward by scaling the rows in the auxilery matrix to some arbitrarily large number so that the relative noise variance is effectively zero.

%\subsection{Other Workloads}  \gm{this needs further development: how do we use the parameterizations for an arbitrary workload? Probably its own section.}

%So far we've discussed and solved the strategy selection problem for (1) arbitrary workloads up to domains of size $ 5000 $, (2) medium dimensional workloads made up of a Kronecker product of sub-workloads, and (3) marginal-like workloads for medium dimensional domains.  In this section, we briefly consider the problem where the domain size is larger than $5000$ and the methods discussed so far do not apply.

%In the 1-dimensional setting, there is not much that can be done without further information about the workload.  However, we propose the following heuristic for large 1D range query workloads: partition the domain into $r$ chunks of tractable size and split up the workload according to this partition $ \W = \begin{bmatrix} \W^{(1)} & \dots & \W^{(r)} \end{bmatrix} $.  Then find $ \A^{(1)}, \dots, \A^{(r)} $ by optimizing for each workload independently and combine them back into a strategy over the full domain by constructing the following block diagonal matrix
%$$ \A = \begin{bmatrix} \A^{(1)} & & \\ & \ddots & \\ & & \A^{(r)} \end{bmatrix} $$
%While this method works well for range-query-like workloads, it may not perform as well for other workloads, as there it is designed for workloads the exhibit strong correlations between nearby cells and weak correlations between distant cells.

%In the multi-dimensional setting, we can ``project'' the workload onto each attribute or disjoint subsets of attributes so that $ \W \approx \W_1 \otimes \dots \otimes \W_d $ then find $ \A_1 \dots, \A_d $ by optimizing on the projected workloads $ \W_1, \dots, \W_d $ and using $ \A = \A_1 \otimes \dots \otimes \A_d $ as the strategy.  We lose information about the workload by applying this projection, so whenever possible it is best to project on subsets of attributes instead of each attribute individually.  For example, if $\W$ is defined over a 6 dimensional domain, we could project $\W$ onto groups of three attributes so that $ \W \approx \W_{123} \otimes \W_{456} $ then optimize accordingly.

\section{Extra experimental results}

\subsubsection*{Distribution of Local Minima}

Because the optimizaiton problem is not convex, we are only able to find locally optimal strategies.  The quality of a locally optimal strategy depends on the initial guess.  We use random initialization, and show the distribution of local minima across $100$ random restarts for two workloads: range queries on a domain of size 256, and up-to-4-way marginals on a domain of size $10^8$.  As shown in figure~\ref{fig:errordist}, the distribution of local minima is very concentrated for the range query workload, indicating that no random restarts are necessary.  The distribution of local minima for the marginals workload varies more, but about 25\% of the local optima were within $1.05$ of the optimal strategy, so only a handful of restarts would be necessary in practice.

\begin{figure}[htb]
\includegraphics[width=\linewidth]{fig/errordist.pdf}
\caption{Empirical distribution of relative error for the locally optimized strategies.}\label{fig:errordist}
\end{figure}

\subsubsection*{Hyper-parameter $p$}

Figure \cref{fig:hyperparam} shows error as function of increasing $p$.

\begin{figure}[htb]
\includegraphics[width=\linewidth]{fig/hyperparam.pdf}
\caption{Empirical distribution of relative error for the locally optimized strategies.}\label{fig:hyperparam}
\end{figure}


\subsubsection*{General Purpose vs. Kronecker Parameterization}

We now compare the General Purpose parameterization with the Kronecker parameterization on a workload of all 2D range queries over a $64 \times 64$ domain.  Solving the optimization problem under the Kronecker parameterization requires optimizing the 1D workload of all range queries over a domain of size $64$.  This is nearly instantaneous, even with thousands of random restarts.  On the other hand, solving the optimization problem under the General purpose parameterization takes some time.  Figure~\ref{fig:kron_vs_general} shows this tradeoff: the General purpose parameterization finds a slightly better strategy, but it takes a few minutes to converge.

\begin{figure}[htb]
\includegraphics[width=\linewidth]{fig/quality_vs_time.pdf}
\caption{Solution quality vs. time for General Purpose Parameterization on all 2D range queries}\label{fig:kron_vs_general}
\end{figure}


\subsection{More results on marginals}

\begin{table}[h]
\centering
\begin{tabular}{c|ccc}
\textbf{k} & \textbf{Identity} & \textbf{Workload} & $\optm$ \\\hline
\textbf{0} & 10000.00          & 1.00              & 1.00         \\
\textbf{1} & 413.91            & 1.00              & 1.00         \\
\textbf{2} & 39.06             & 1.00              & 1.00         \\
\textbf{3} & 7.13              & 1.11              & 1.00         \\
\textbf{4} & 2.05              & 1.21              & 1.00         \\
\textbf{5} & 1.01              & 1.47              & 1.00         \\
\textbf{6} & 1.00              & 2.29              & 1.00         \\
\textbf{7} & 1.00              & 2.14              & 1.00         \\
\textbf{8} & 1.00              & 1.00              & 1.00
\end{tabular}
\caption{Relative RMSE on the workload of all $k$-way marginals for a domain of size $ 10^8 $} \label{table:marginals2}
\end{table}

\subsection*{Strategy visualization}
\begin{figure}
\includegraphics[width=\linewidth]{fig/viz256.pdf}
\end{figure}

To provide some insight into the solutions found by $\optgp$ we show a visualization of the output of $\optgp$ in Figure~\ref{fig:range_strategy}, which shows an understandable structure, but, interestingly, one that is not consistent with the hierarchical structures common to many heuristic strategy selection methods.  The visualization illustrates each of the rows of the $p=13$ non-Identity queries in the output of $\optgp$, when optimizing the workload $R$ of all range queries on a domain of size 256.  The $x$-axis represents the cells in the data vector and the $y$-axis represents the weight on that cell in the query.  The identity queries are not plotted, since weights on those queries can be derived from the non-Identity weights.  %It is unfortunately difficult to visualize higher-dimensional strategies produced by \sys.

% for the workload of all range queries, the strategy produced by the optimization has an understandable structure.  shows a visual representation of the strategy, on a domain of size 256.
